# Supplementary material for: In-Context Principle Learning from Mistakes
Source: arXiv:2402.05403 source file (2024-02-09)
Supplement: Supplementary file 1 [file prompts.tex]

\section{Prompts}
\label{sec:prompts}

\begin{figure}[b]
\begin{tcolorbox}
Can you summarize common mistakes from the following mistakes and correct answers. Then provide a guideline contain general rules you learned from the correct solution that is useful for the solving the similar type of problems correctly.
% Tianjun: please check if there's a typo hereSome incorrect answers might just because the formatting is not compatible." + question + " 
Your final answer should be in for format of:
Mistake: \{mistake\}
Guideline: \{guideline\}
Reason: \{reason\}
\end{tcolorbox}
\caption{Prompt for learning high-level principle}
\end{figure}

\begin{figure}[b]
\begin{tcolorbox}
Always ensure that the final answer is in the correct format as specified in the question. In this case, the final answer should be a single numerical number, in the form \boxed{answer}, at the end of your response.
Always double-check your calculations and make sure you understand the problem correctly. Break down the problem into smaller parts if necessary.
Always explain your reasoning clearly and step by step. This helps the reader understand how you arrived at the final answer.
\end{tcolorbox}
\begin{tcolorbox}
 Always provide the final answer in the form of a single numerical number, in the form \\boxed{answer}, at the end of your response.
Always read the problem carefully and understand what is being asked before attempting to solve it. Break down the problem into smaller parts if necessary.
Always show all the steps in your calculation, even if some steps seem obvious. This helps to ensure that you have not made any mistakes and makes it easier for others to follow your reasoning.
Always check your answer to make sure it makes sense in the context of the problem. If your answer seems unreasonable, you may have made a mistake in your calculations.
\end{tcolorbox}
\caption{\textbf{Prompts for GSM8K}: The prompt used for GSM8K}
\label{fig:gsm8k}
\end{figure}

\begin{figure}[b]
\begin{tcolorbox}
 The standard form of a circle's equation is $(x-h)^2 + (y-k)^2 = r^2$, where $(h,k)$ is the center of the circle and $r$ is the radius. To find the center of a circle given its equation in general form, you need to complete the square for the $x$ and $y$ terms and rewrite the equation in standard form.
 When solving a system of equations, it's important to correctly identify the equations from the problem and solve them accurately. In this problem, the student should have recognized that the differences between consecutive terms in an arithmetic sequence are constant, and used this property to set up and solve the system of equations.
 When solving an inequality, it's important to correctly manipulate the inequality and consider all possible cases. In this problem, the student should have recognized that the inequality holds for all values of $p$ except for $p=-3$ and $q=\frac{1}{4}$, and used this information to correctly solve the inequality.
 When using the compound interest formula, it's important to correctly substitute the given values into the formula and perform the calculations accurately. The formula for compound interest is $A = P \left(1 + \frac{r}{n}\right)^{nt}$, where $A$ is the future value of the investment, $P$ is the principal amount (the initial amount of money), $r$ is the annual interest rate (in decimal form), $n$ is the number of times that interest is compounded per year, and $t$ is the time the money is invested for, in years.
 \end{tcolorbox}
 \caption{\textbf{Prompts for MATH}: The prompt used for Competitive Math}
\label{fig:math}
 \end{figure}
