# Supplementary material for: In-Context Principle Learning from Mistakes
Source: arXiv:2402.05403 source file (2024-02-09)
Supplement: Supplementary file 2 [file non_cot_bbh_results.tex]

% \section{\ours without \cotp}
% \label{sec:appendix:ours_without_cotp}

% % \todo{aman}
% \aman{todo}
